# Supplementary material for: HyperStyle: StyleGAN Inversion with HyperNetworks for Real Image Editing
Source: arXiv:2111.15666 source file (2022-03-29)
Supplement: Supplementary file 7 [file face_editings_styleclip.tex]

\begin{figure*}

    \setlength{\tabcolsep}{1pt}
    \centering
    { \small
    \begin{tabular}{c c | c c c c c}

    \includegraphics[width=0.12\linewidth]{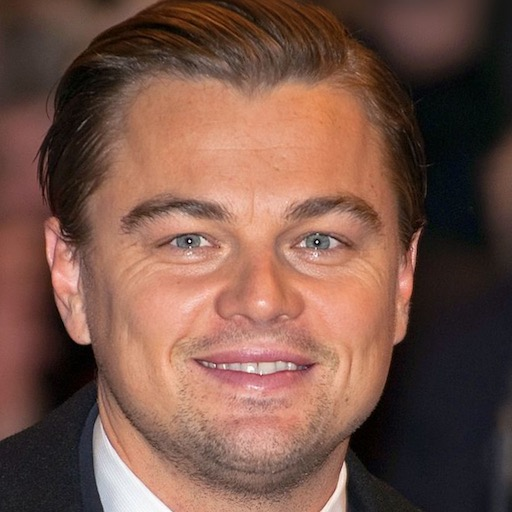} &
    \includegraphics[width=0.12\linewidth]{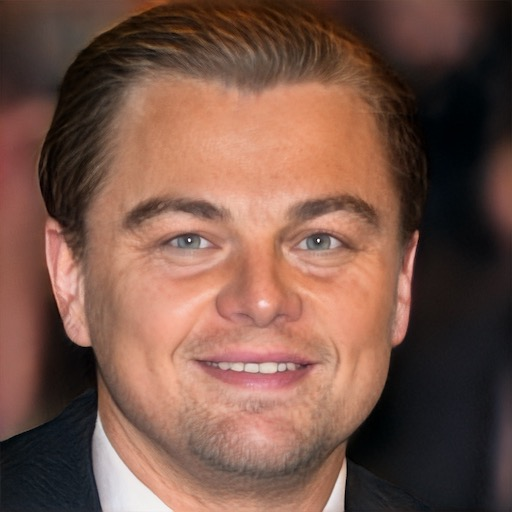} &
    \includegraphics[width=0.12\linewidth]{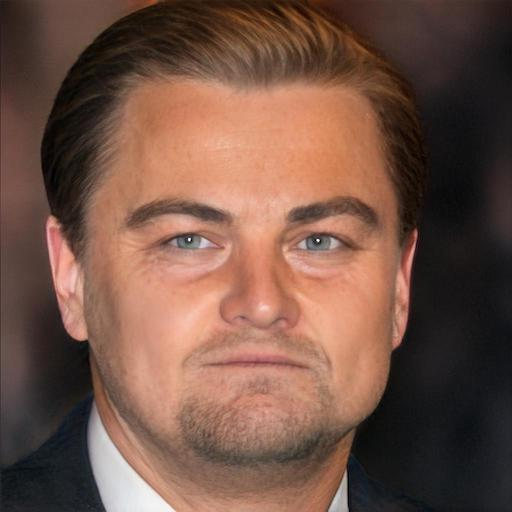} &
    \includegraphics[width=0.12\linewidth]{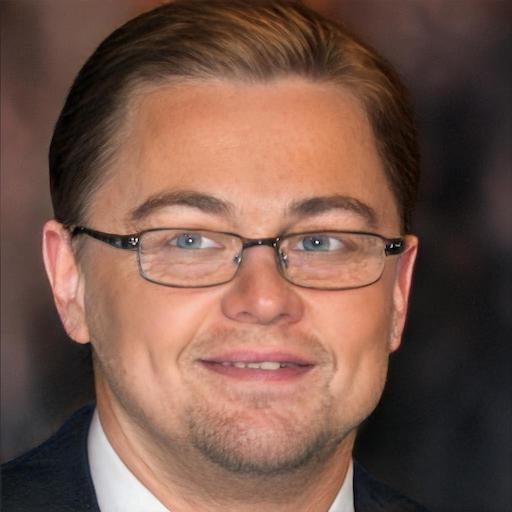} &
    \includegraphics[width=0.12\linewidth]{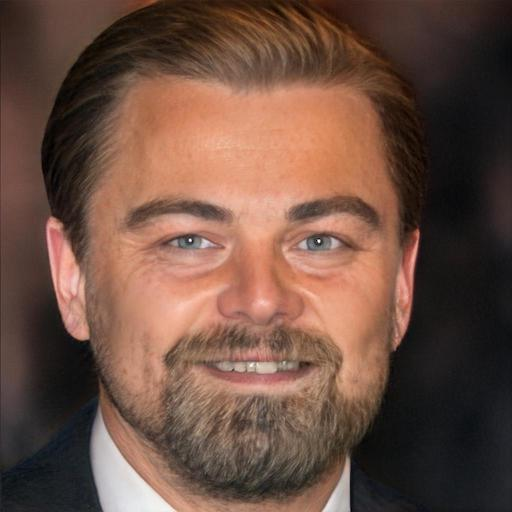} &
    \includegraphics[width=0.12\linewidth]{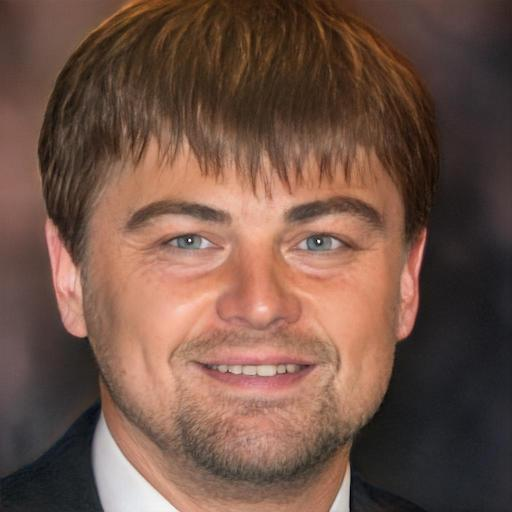} &
    \includegraphics[width=0.12\linewidth]{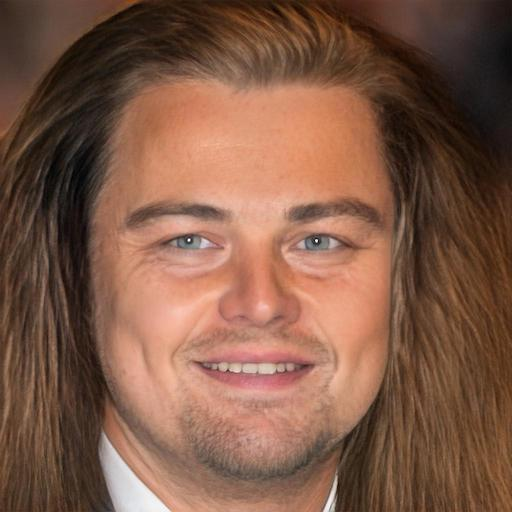} \\
    
    Input & Inversion & Sad & Glasses & Beard & Bowl Cut & Long Hair \\

    \includegraphics[width=0.12\linewidth]{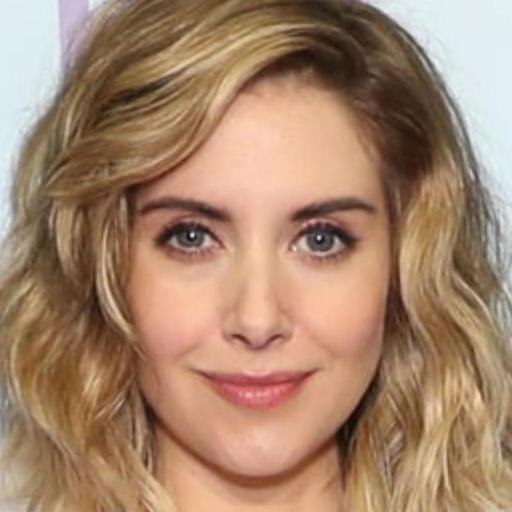} &
    \includegraphics[width=0.12\linewidth]{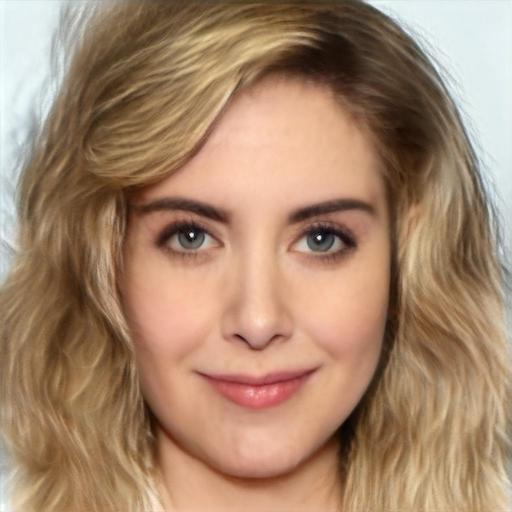} &
    \includegraphics[width=0.12\linewidth]{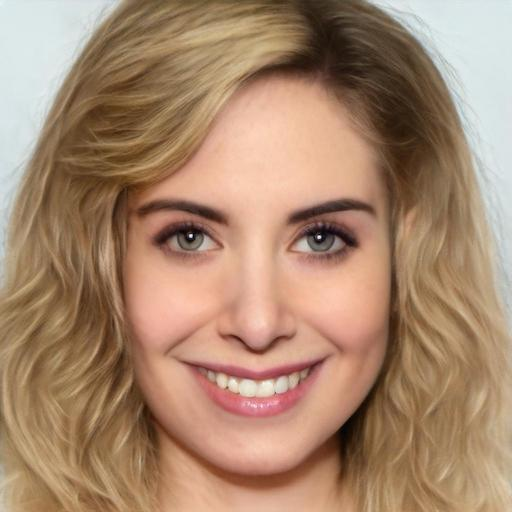} &
    \includegraphics[width=0.12\linewidth]{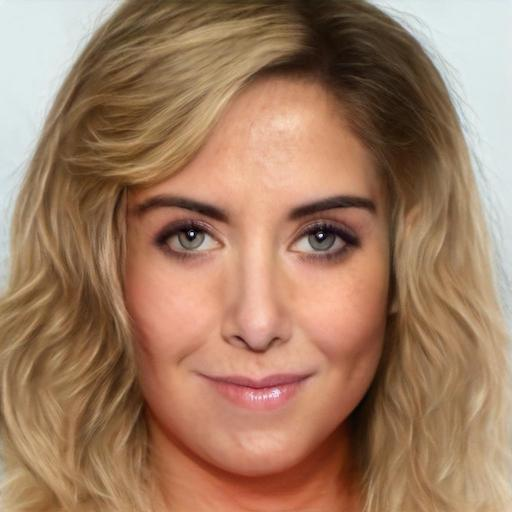} &
    \includegraphics[width=0.12\linewidth]{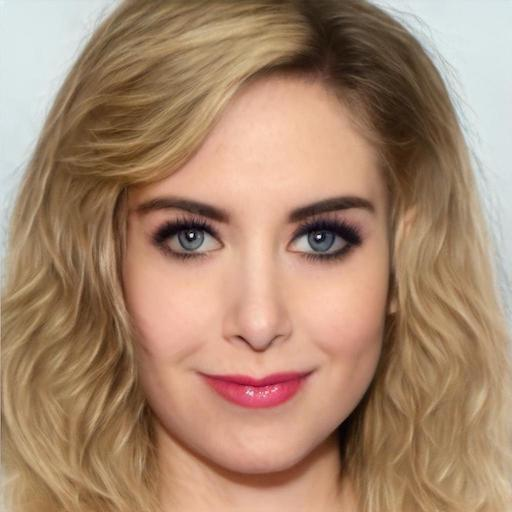} &
    \includegraphics[width=0.12\linewidth]{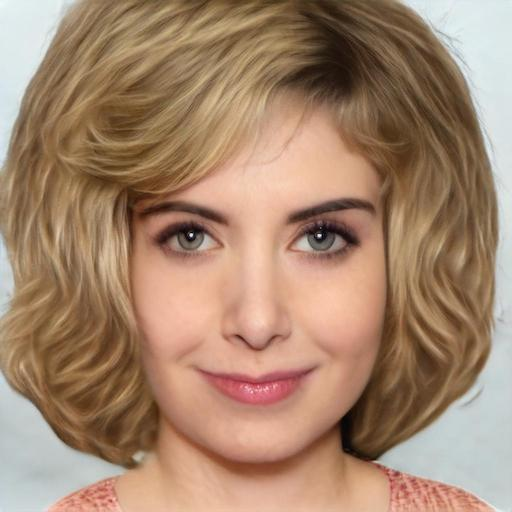} &
    \includegraphics[width=0.12\linewidth]{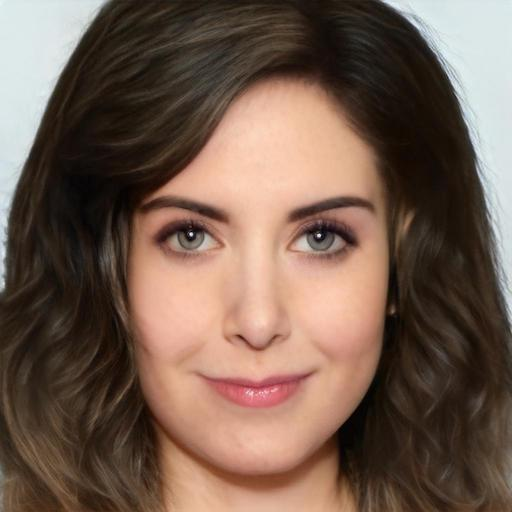} \\
    
    Input & Inversion & Smile & Tanned & Makeup & Short Hair & Brown Hair \\
    
    \includegraphics[width=0.12\linewidth]{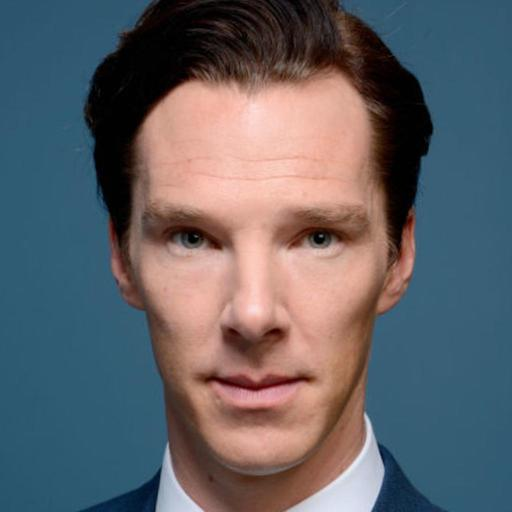} &
    \includegraphics[width=0.12\linewidth]{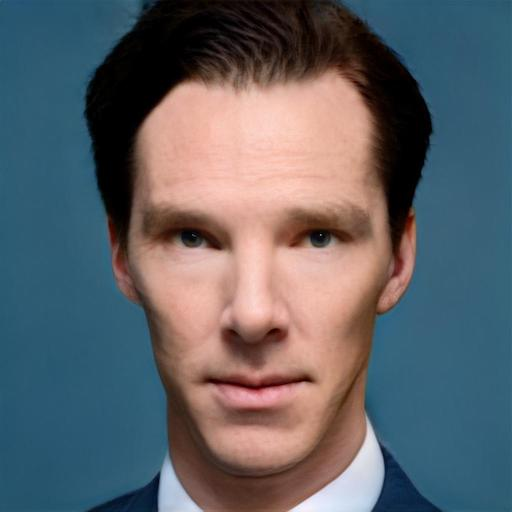} &
    \includegraphics[width=0.12\linewidth]{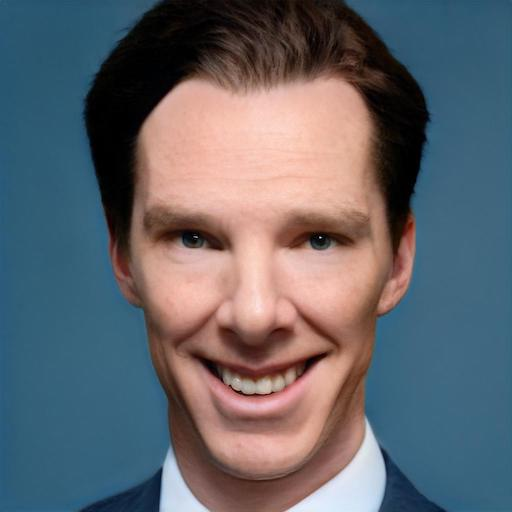} &
    \includegraphics[width=0.12\linewidth]{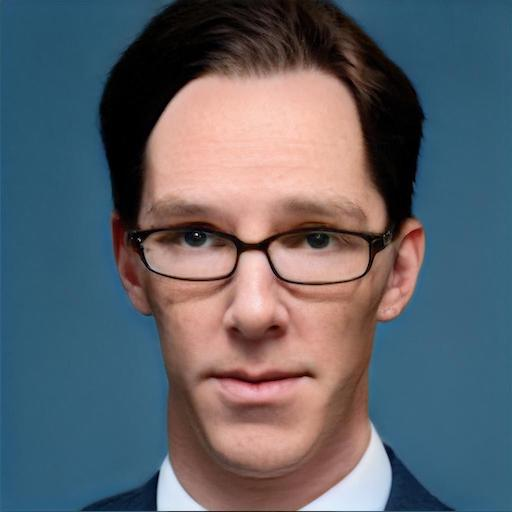} &
    \includegraphics[width=0.12\linewidth]{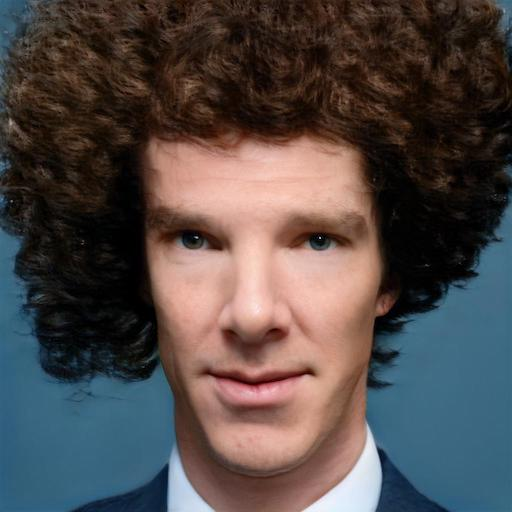} &
    \includegraphics[width=0.12\linewidth]{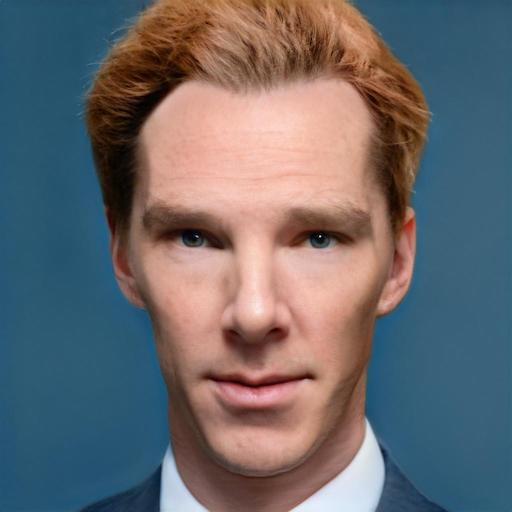} &
    \includegraphics[width=0.12\linewidth]{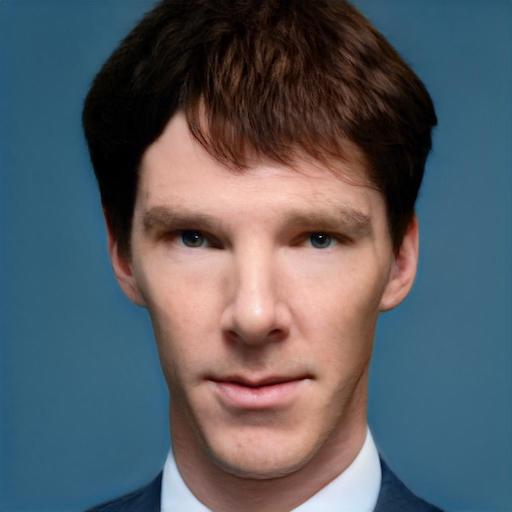} \\
    
    Input & Inversion & Smile & Glasses & Afro & Blonde Hair & Bowl Cut \\
    
    \includegraphics[width=0.12\linewidth]{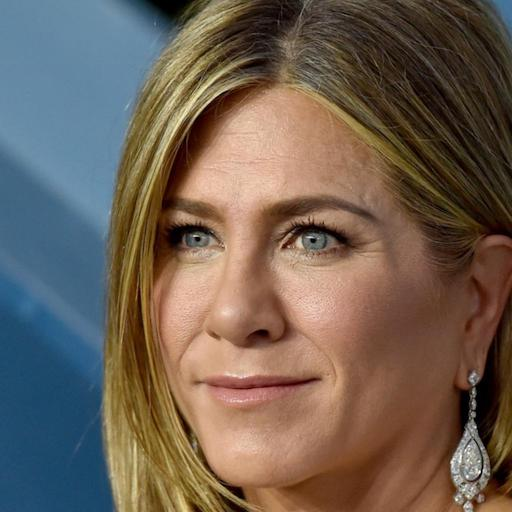} &
    \includegraphics[width=0.12\linewidth]{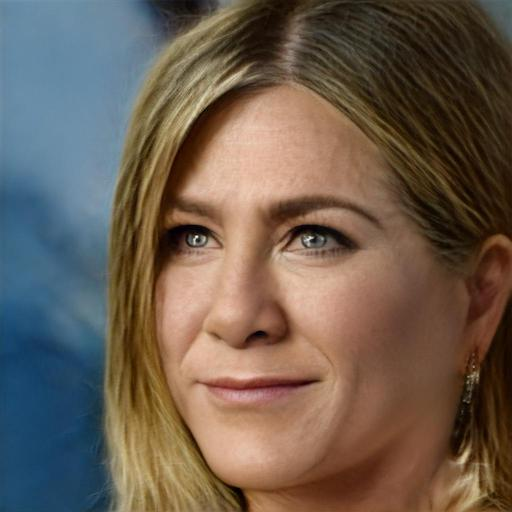} &
    \includegraphics[width=0.12\linewidth]{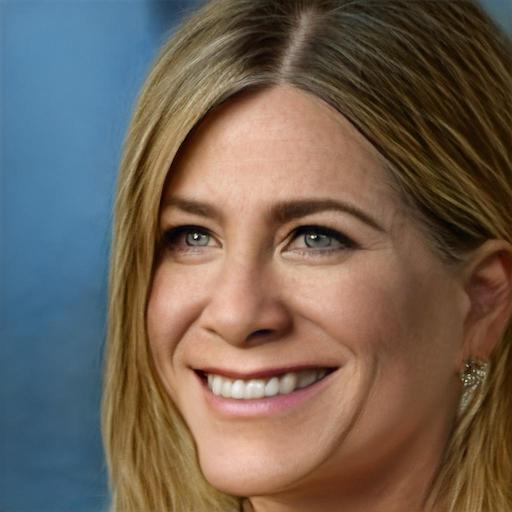} &
    \includegraphics[width=0.12\linewidth]{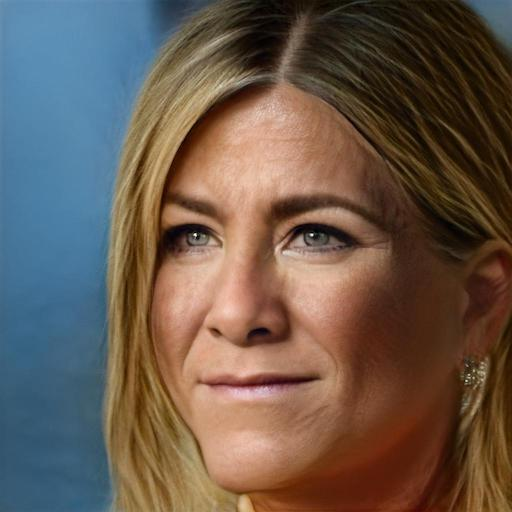} &
    \includegraphics[width=0.12\linewidth]{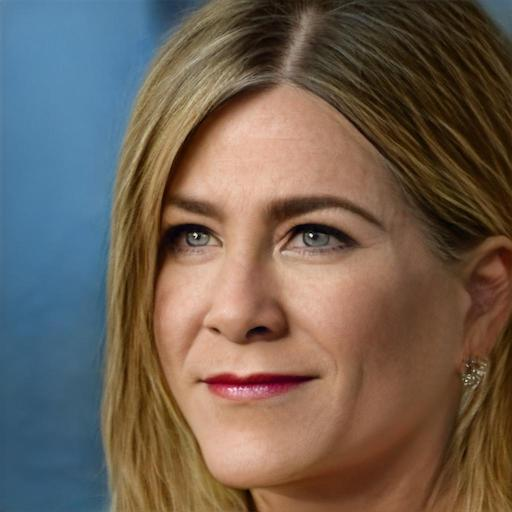} &
    \includegraphics[width=0.12\linewidth]{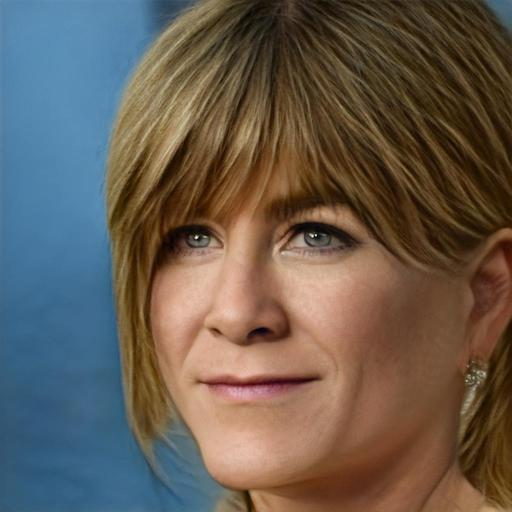} &
    \includegraphics[width=0.12\linewidth]{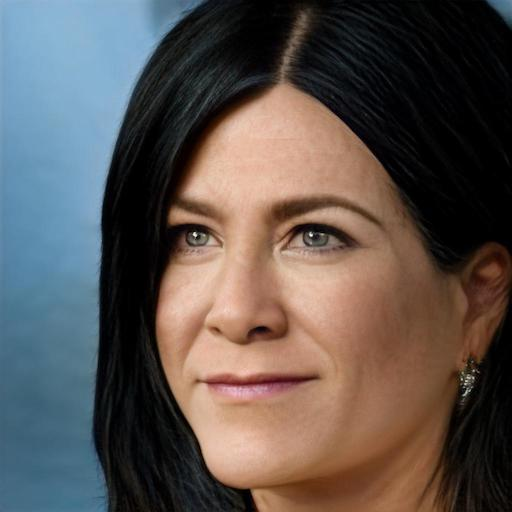} \\
    
    Input & Inversion & Smile & Tanned & Lipstick & Bob Cut & Black Hair \\
    
    \includegraphics[width=0.12\linewidth]{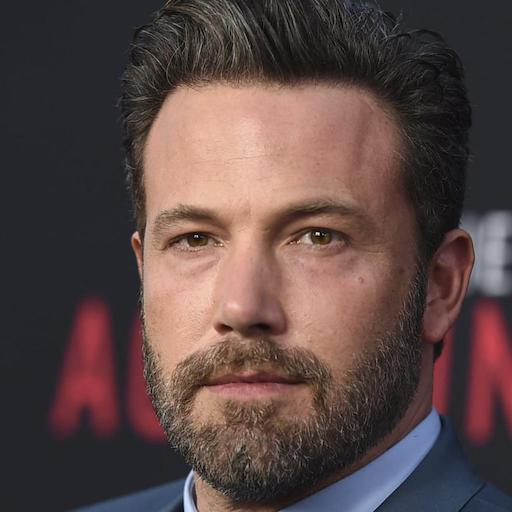} &
    \includegraphics[width=0.12\linewidth]{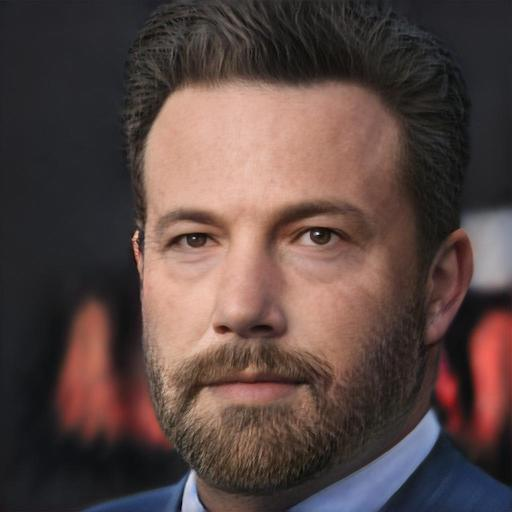} &
    \includegraphics[width=0.12\linewidth]{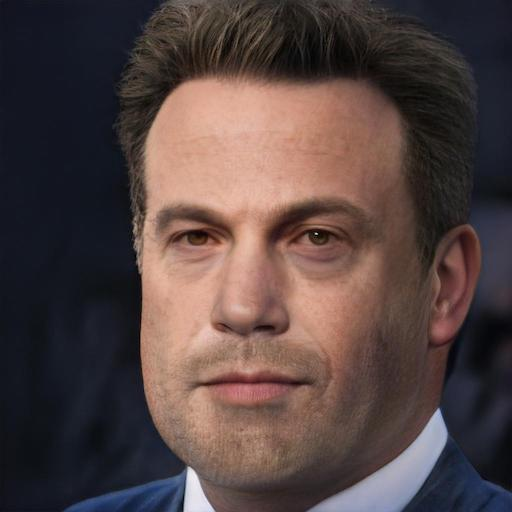} &
    \includegraphics[width=0.12\linewidth]{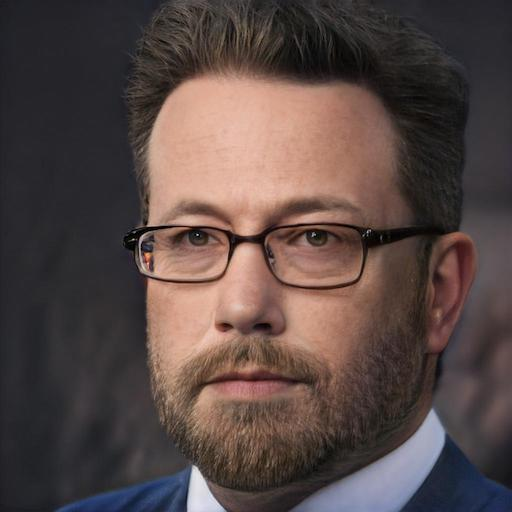} &
    \includegraphics[width=0.12\linewidth]{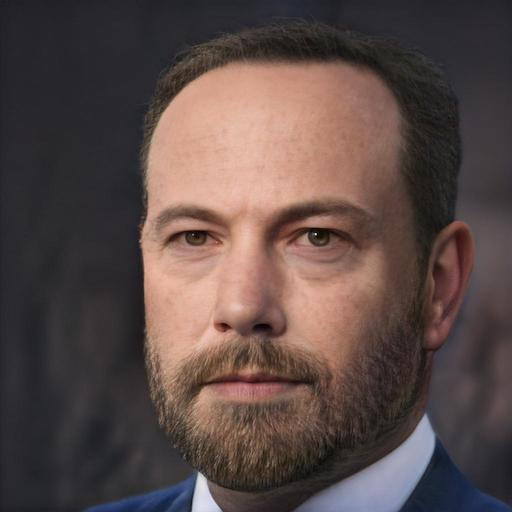} &
    \includegraphics[width=0.12\linewidth]{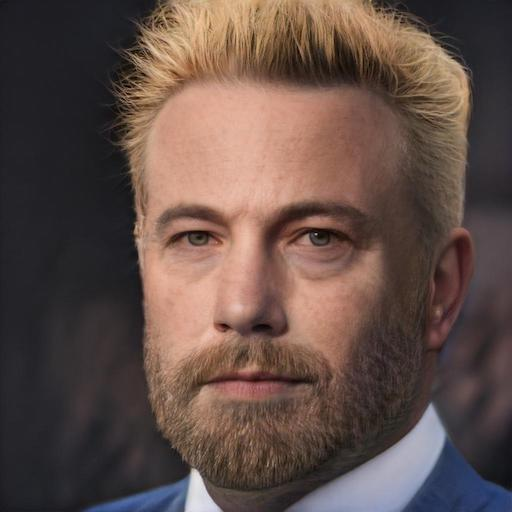} &
    \includegraphics[width=0.12\linewidth]{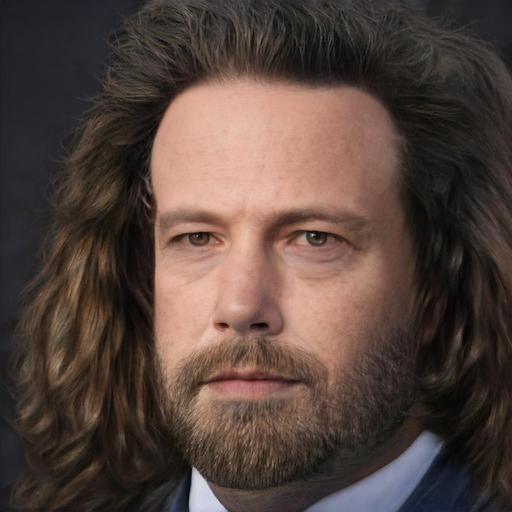} \\
    
    Input & Inversion & No Beard & Glasses & Bald & Blonde Hair & Long Hair \\
    
    \includegraphics[width=0.12\linewidth]{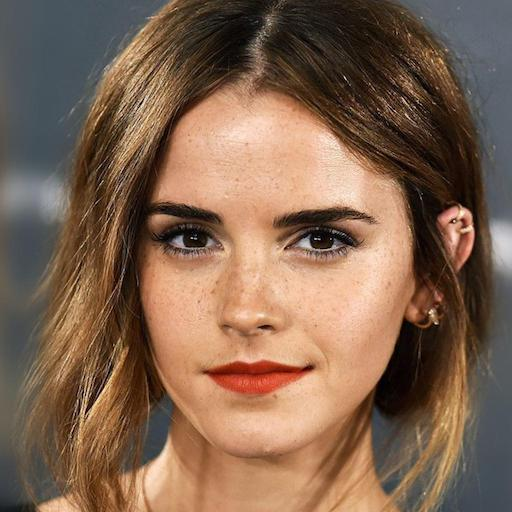} &
    \includegraphics[width=0.12\linewidth]{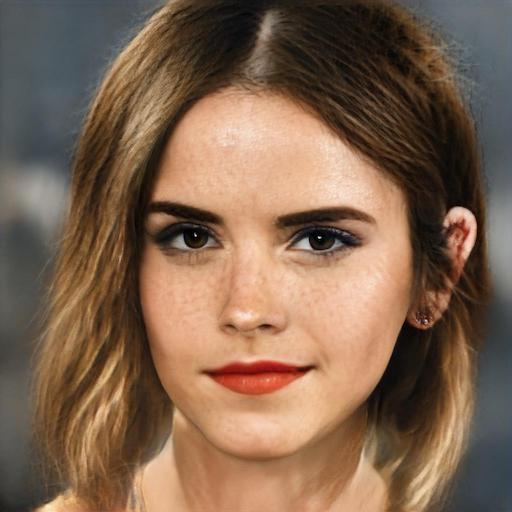} &
    \includegraphics[width=0.12\linewidth]{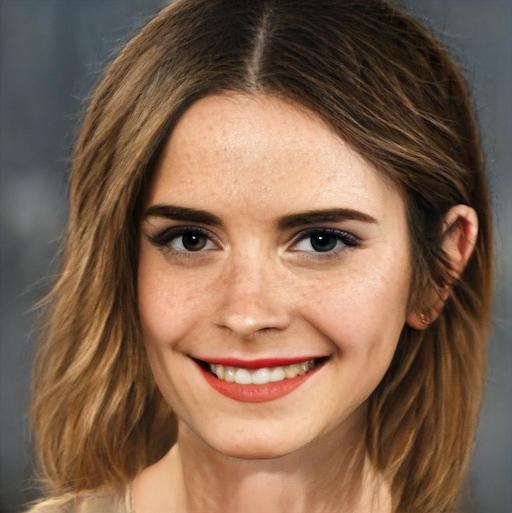} &
    \includegraphics[width=0.12\linewidth]{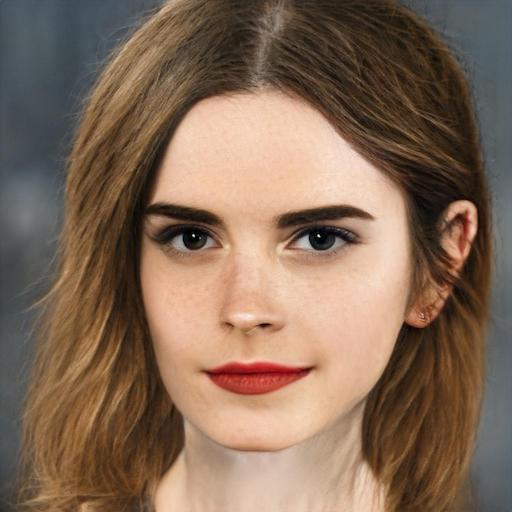} &
    \includegraphics[width=0.12\linewidth]{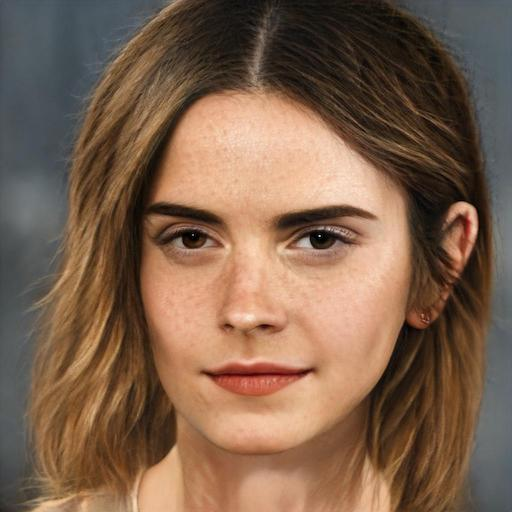} &
    \includegraphics[width=0.12\linewidth]{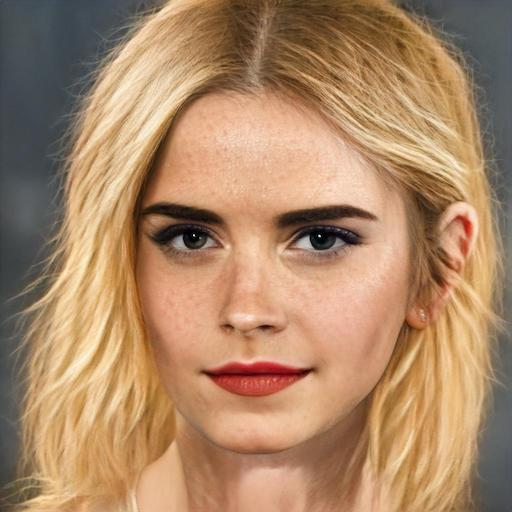} &
    \includegraphics[width=0.12\linewidth]{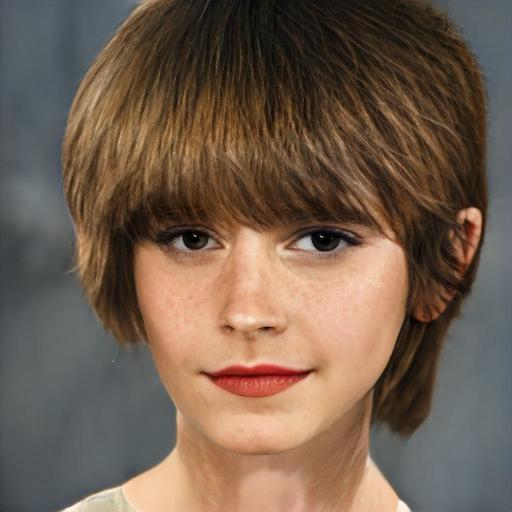} \\
    
    Input & Inversion & Smile & Pale & No Makeup & Blonde Hair & Bowl Cut \\
    
    \includegraphics[width=0.12\linewidth]{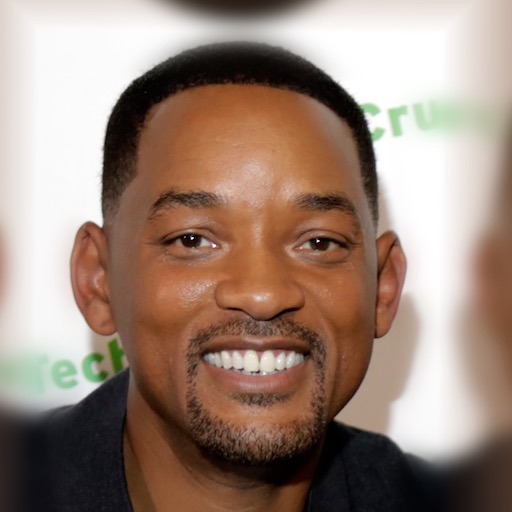} &
    \includegraphics[width=0.12\linewidth]{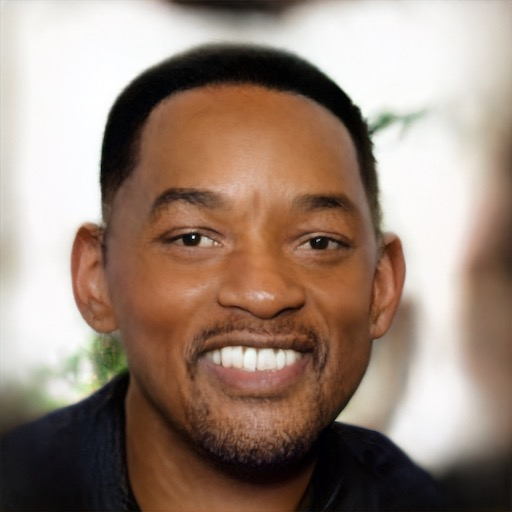} &
    \includegraphics[width=0.12\linewidth]{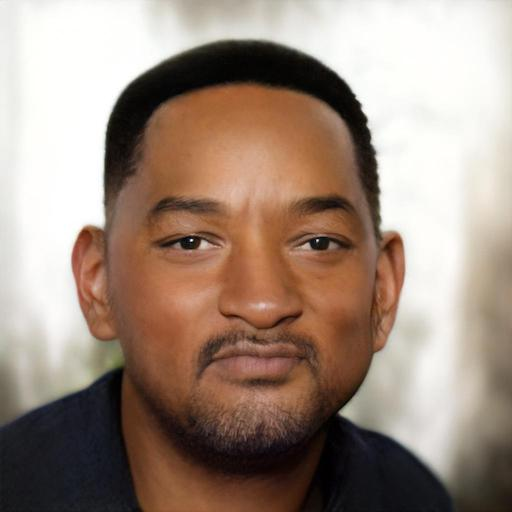} &
    \includegraphics[width=0.12\linewidth]{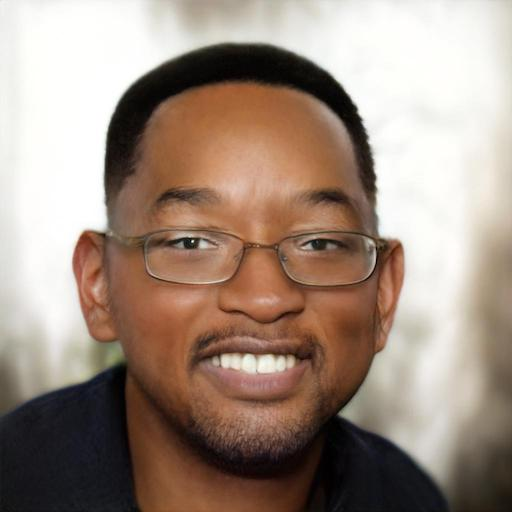} &
    \includegraphics[width=0.12\linewidth]{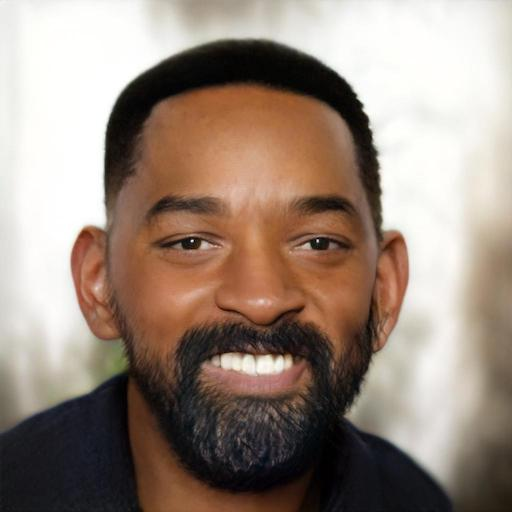} &
    \includegraphics[width=0.12\linewidth]{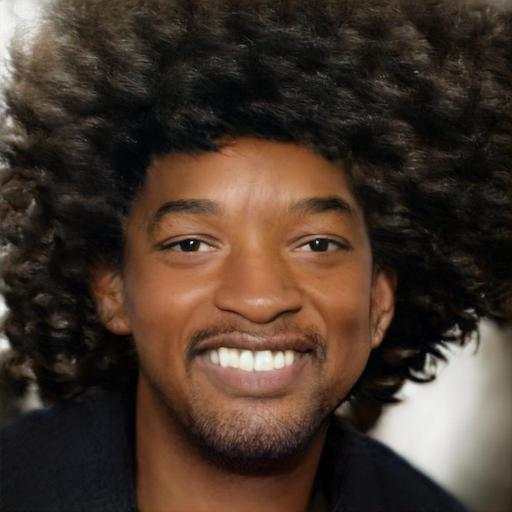} &
    \includegraphics[width=0.12\linewidth]{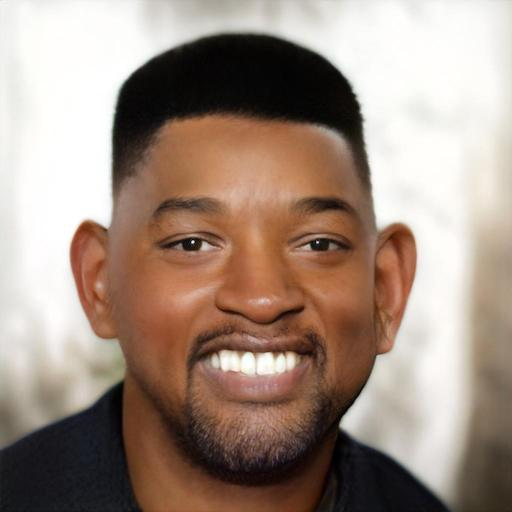} \\

    Input & Inversion & Sad & Glasses & Beard & Afro & Hi-Top Fade \\
    
    \includegraphics[width=0.12\linewidth]{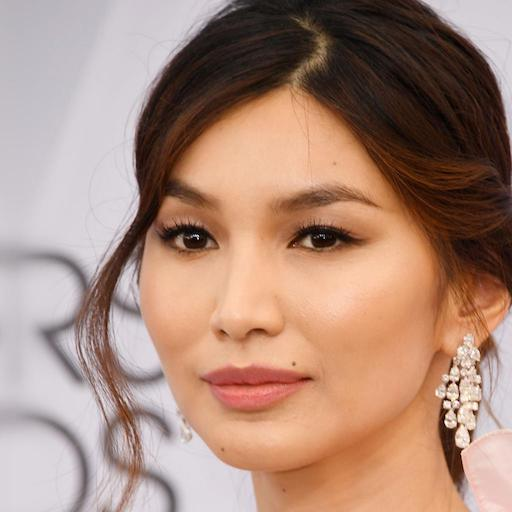} &
    \includegraphics[width=0.12\linewidth]{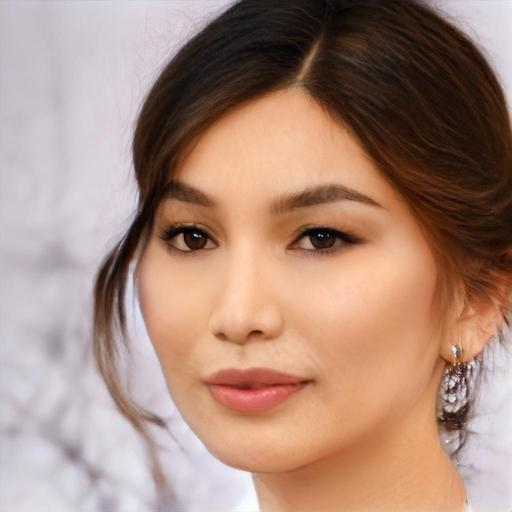} &
    \includegraphics[width=0.12\linewidth]{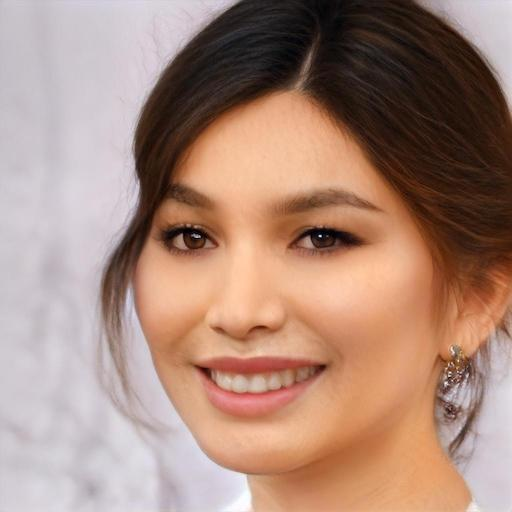} &
    \includegraphics[width=0.12\linewidth]{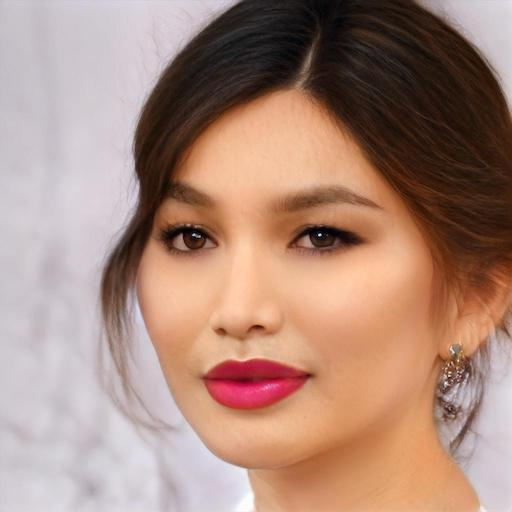} &
    \includegraphics[width=0.12\linewidth]{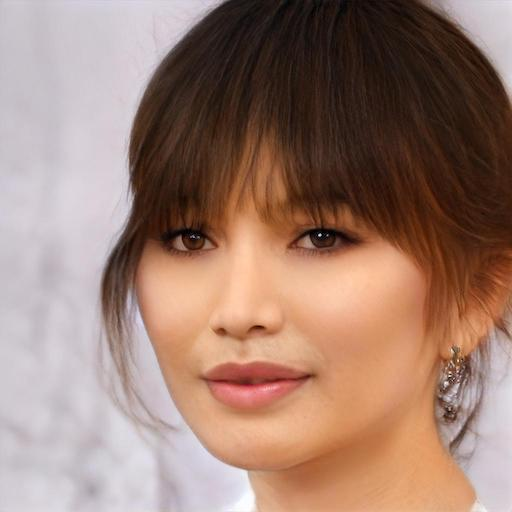} &
    \includegraphics[width=0.12\linewidth]{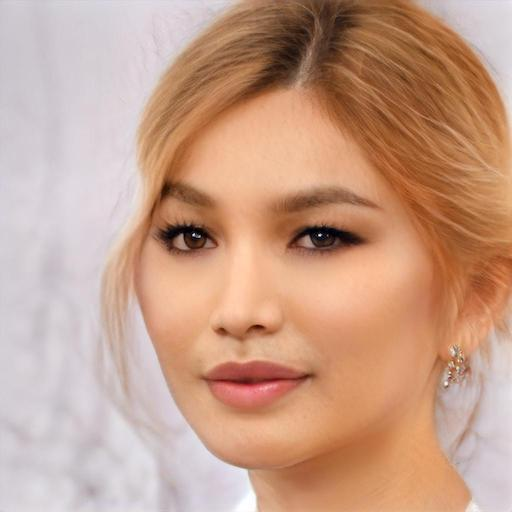} &
    \includegraphics[width=0.12\linewidth]{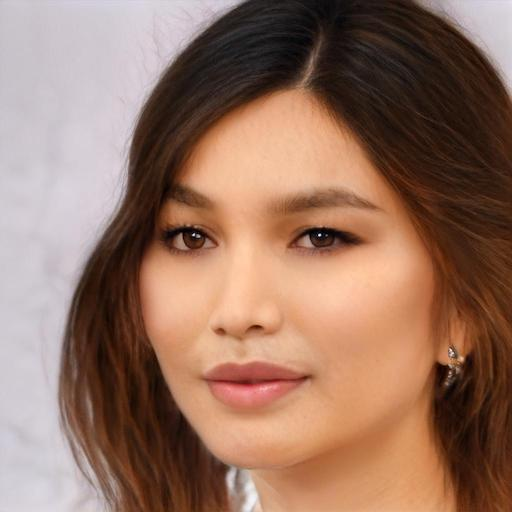} \\

    Input & Inversion & Smile & Lipstick & Bangs & Blonde Hair & Long Hair \\

    \end{tabular}
    }
    \caption{Additional reconstruction and editing results obtained by HyperStyle over the facial domain using StyleCLIP's~\cite{shen2020interpreting} global direction approach. We illustrate a wide range of edits including changes to expression, facial hair, makeup, and hairstyle.}
    \label{fig:supp_face_editings_styleclip}
\end{figure*}
